# Supplementary material for: An automata characterisation for multiple context-free languages
Source: arXiv:1606.02975 source file (2016-09-23)
Supplement: Supplementary file 1 [file supplemental-proofs.tex]

\section{Supplemental Proofs}

%%% Local Variables:
%%% mode: latex
%%% TeX-master: "ta"
%%% End:
